# Supplementary material for: Legal Question-Answering in the Indian Context: Efficacy, Challenges, and Potential of Modern AI Models
Source: arXiv:2309.14735 source file (2023-10-16)
Supplement: Supplementary file 1 [file appendix.tex]

% \newpage
% \clearpage
\appendix
\section{Appendix}
\label{sec:appendix}

% \begin{figure}
%     \centering
%     \includegraphics[width=\textwidth]{figures/BM25_OpenAI_flowdiagram.pdf}
%     \caption{The Diagrammatic Representation of the Question-Answering Framework: Extracting Relevant Documents from the Corpus via BM25 and Generating Answers with OpenAI GPT-3 LLM Model, Augmented with Relevant Prompts.}
%     \label{fig:bm25_openai_flowdiagram}
% \end{figure}

% \begin{table}[htbp]
% \caption{List of Acts}
% \centering
% \begin{tabular}{|c|l|}
% \hline
% \textbf{S.No.} & \textbf{Act} \\
% \hline
% 1 & Indian Penal Code \\
% 2 & Protection of Children from Sexual Offences Act \\
% 3 & Criminal Procedural Code \\
% 4 & Indian Evidence Act \\
% 5 & Arms Act \\
% 6 & Information Technology Act \\
% 7 & Narcotic Drugs and Psychotropic Substances Act \\
% 8 & Contempt of Courts Act \\
% 9 & Unlawful Activities Prevention Act \\
% 10 & Prevention of Money Laundering Act \\
% 11 & Criminal Procedure Identification Act \\
% 12 & Extradition Act of 1962 \\
% 13 & Prisons Act of 1894 \\
% 14 & Prevention of Corruption Act of 1988 \\
% 15 & Gram Nyayalayas Act of 2008 \\
% \hline
% \end{tabular}
% \label{appendix:list_of_acts}
% \end{table}
%%%%%%%%%%%%%%%%%%%%%%%%%%%%%%%%%%%%%%%%%%%%%%%
% \begin{figure*}[h!]
%     \centering
%     \includegraphics[width=\textwidth]{figures/density_plot.pdf}
%     \caption{It is a plot between MPNET similarity score vs Density of the questions falling in that score.}
%     \label{fig:density_plot}
% \end{figure*}
%%%%%%%%%%%%%%%%%%%%%%%%%%%%%%%%%%%%%%%%%%%%%%%

%%%%%%%%%%%%%%%%%%%%%%%%%%%%%%%%%%%%%%%%%%%%%%%%%%%%%%%%%%%%
